# Supplementary material for: Capacity Allocation and Pricing of High Occupancy Toll Lane Systems with Heterogeneous Travelers
Source: arXiv:2304.09234 source file (2024-12-03)
Supplement: Supplementary file 1 [file appendix.tex]

\subsection{Proof of Theorem \eqref{thm:NE}}
In all proofs, we denote the uniform preference parameter distribution as \[f(\beta, \gamma) = \frac{1}{\bar{\beta}\bar{\gamma}}.\]
\begin{proof}
    In each regime, we first show that the desired equation has a unique fixed point and then show that the solution $(\sigma^*_{toll}, \sigma^*_{pool}, \sigma^*_{o})$ indeed satisfies the equilibrium condition \ref{eq: equilibrium condition}.

    \medskip 
    \noindent \underline{Regime $A$}: 
    \begin{enumerate}
        \item $\ugamma > \ubeta C_\delta(0, \frac{\tau}{2\ugamma}, 1 - \frac{\tau}{2\ugamma}; \rho) $.

        Combine $\ugamma > \ubeta C_\delta(0, \frac{\tau}{2\ugamma}, 1 - \frac{\tau}{2\ugamma}; \rho) $ with the regime condition $\tau > \min\left\{\ugamma,~ \ubeta C_\delta\left(0, \frac{\tau}{2\bar \gamma}, 1 -  \frac{\tau}{2\bar \gamma}, \rho\right)\right\}$, we have $$\tau > \ubeta C_\delta(0, \frac{\tau}{2\ugamma}, 1 - \frac{\tau}{2\ugamma}; \rho).$$

        First, we need to show that equation \ref{eq:b2-fixed_point1}
        \begin{align*}
            \frac{1}{2} \frac{\ubeta}{\ugamma} C_\delta(0, \sigma_{pool}, 1 - \sigma_{pool}; \rho) = \sigma_{pool}
        \end{align*} has a unique fixed point.

        Let $$f(\sigma_{pool}) = \frac{\sigma_{pool}}{C_\delta(0, \sigma_{pool}, 1 - \sigma_{pool}; \rho)}.$$

        Recall that $C_\delta(\sigma; \rho) = C_o(\sigma_{o} D; 1 - \rho) - C_h((\sigma_{toll} + \frac{\sigma_{pool}}{A})D; \rho)$,  and that $C_o(x_o; 1 - \rho)$ and $C_h(x_h; \rho)$ are increasing in $x_o, x_h$. Then, $C_\delta(0, \sigma_{pool}, 1 - \sigma_{pool}; \rho)$ is decreasing in $\sigma_{pool}$ and $f(\sigma_{pool})$ is increasing in $\sigma_{pool}$.

        Since $\tau> \ubeta C_\delta(0, \frac{\tau}{2\ugamma}, 1 - \frac{\tau}{2\ugamma}; \rho) $, $$f(\frac{\tau}{2\ugamma}) = \frac{\frac{\tau}{2\ugamma}}{C_\delta(0, \frac{\tau}{2\ugamma}, 1 - \frac{\tau}{2\ugamma}; \rho)} > \frac{\ubeta}{2\ugamma}.$$

        %Notice any solution to the equation \ref{eq:b2-fixed_point1} must satisfies $$f(\sigma) = \frac{\sigma}{C_\delta(0, \sigma, 1 - \sigma; \rho)} = \frac{\ubeta}{2\ugamma}.$$

        Since we also have $f(0) = 0$, by the continuity and monotonicity of $f$, there exists a unique $\sigma_{pool}^*$ such that $$f(\sigma_{pool}^*) = \frac{\sigma_{pool}^*}{C_\delta(0, \sigma_{pool}^*, 1 - \sigma_{pool}^*; \rho)} = \frac{\ubeta}{2\ugamma},$$
        which is the fixed point of equation \ref{eq:b2-fixed_point1}. Moreover, $\sigma_{pool}^* < \frac{\tau}{2\ugamma}$.

        Now it suffices to show that $\sigma^*_{toll} = 0, \sigma^*_{pool}, \sigma^*_{o} = 1 - \sigma^*_{pool}$ satisfy the equilibrium condition \ref{eq: equilibrium condition}.

        Notice $$\tau > 2 \ugamma \sigma_{pool}^* = \ubeta C_\delta\left(0,\sigma_{pool}^*,1-\sigma_{pool}^*;\rho\right),$$ where the inequality follows from $\sigma_{pool}^* < \frac{\tau}{2\ugamma}$ and the equality follows from equation \ref{eq:b2-fixed_point1}.
        
        Therefore, \begin{align*}
            c^\beta_\gamma(R_{toll}) &= \beta \cdot C_h\left(\left(\sigma_{toll} + \frac{\sigma_{pool}}{A}\right)D; \rho\right) + \tau \\ &> \beta \cdot C_o(\sigma_{o} D; 1 - \rho) = c^\beta_\gamma(R_o; \sigma)
        \end{align*} for all $\beta \in [0,\ubeta]$ and $\gamma \in [0, \ugamma]$. That is, the cost of paying the HOT toll price will be higher than taking the ordinary lane for all agents. Hence, nobody will choose $R_{toll}$ and $\sigma^*_{toll} = 0$ satisfies the equilibrium condition \ref{eq: equilibrium condition}. Since $\sigma^*_{toll} + \sigma^*_{pool} + \sigma^*_{o} = 0$, we also have $\sigma^*_{o} = 1 - \sigma^*_{pool}$.

        An agent $(\beta,\gamma)$ will choose $R_{poll}$ over $R_{o}$ if $c^\beta_\gamma(R_{pool}; \sigma) < c^\beta_\gamma(R_o; \sigma)$, which is equivalent to $\gamma < \beta C_\delta(0, \sigma^*_{pool}, \sigma^*_{o}; \rho)$. Thus, $R_{pool}  = \{(\beta, \gamma) : 0 < \beta < \ubeta, 0 < \gamma < \beta C_\delta(0, \sigma^*_{pool})\}$.

        Notice also $D = \ubeta \ugamma f(\beta, \gamma)$, then equation \ref{eq:b2-fixed_point1} is equivalent to  $$\int_{0}^{\ubeta}\int_{0}^{\beta C_\delta(0, \sigma^*_{pool}, \sigma^*_{o}; \rho)} f(\beta, \gamma) d\gamma d\beta = D \sigma^*_{pool}.$$

        Therefore, $\sigma^*_{pool}$ and $\sigma^*_{o} = 1 - \sigma^*_{pool}$ satisfies the equilibrium condition \ref{eq: equilibrium condition}.
        
        \item  $\ugamma < \ubeta C_\delta(0, \frac{\tau}{2\ugamma}, 1 - \frac{\tau}{2\ugamma}; \rho)$. 
        
        Combine $\ugamma < \ubeta C_\delta(0, \frac{\tau}{2\ugamma}, 1 - \frac{\tau}{2\ugamma}; \rho) $ with the regime condition $\tau > \min\left\{\ugamma,~ \ubeta C_\delta\left(0, \frac{\tau}{2\bar \gamma}, 1 -  \frac{\tau}{2\bar \gamma}, \rho\right)\right\}$, we have $$\tau > \ugamma.$$
        
        First, we need to show that equation \ref{eq:b2-fixed_point2}
        $$
            \frac{1}{2} \frac{\ugamma}{\ubeta} \frac{1}{C_\delta(0, \sigma_{pool}, 1 - \sigma_{pool}; \rho)} = 1 - \sigma_{pool}
        $$ has a unique fixed point.

        Let $$g(\sigma_{pool}) = C_\delta(0, \sigma_{pool}, 1 - \sigma_{pool}; \rho) (1 - \sigma_{pool})$$

        Notice $g$ is continuous and decreasing in $\sigma_{pool}$ and $g(1) = 0$.

        Furthermore, \begin{align*}
            g(\frac{\tau}{2\ugamma}) &= C_\delta(0, \frac{\tau}{2\ugamma}, 1 - \frac{\tau}{2\ugamma}; \rho) (1 - \frac{\tau}{2\ugamma}) \\
            &> \frac{\ugamma}{\ubeta}(1 - \frac{\tau}{2\ugamma}) \qquad \text{(Since } \ugamma < \ubeta C_\delta(0, \frac{\tau}{2\ugamma}, 1 - \frac{\tau}{2\ugamma}; \rho))\\
            &>\frac{\ugamma}{\ubeta}(1 - \frac{\ugamma}{2\ugamma})  \qquad \text{(Since } \tau > \ugamma)\\ 
            &= \frac{\ugamma}{2\ubeta}
        \end{align*}

        By the continuity and monotonicity of $g$, there exists a unique $\sigma_{pool}^*$ such that $$g(\sigma^*_{pool}) = C_\delta(0, \sigma^*_{pool}, 1 - \sigma^*_{pool}; \rho) (1 - \sigma^*_{pool}) = \frac{\ugamma}{2\ubeta},$$
        which is the fixed point of equation \ref{eq:b2-fixed_point2}. Moreover, $\sigma_{pool}^* > \frac{\tau}{2\ugamma}$.

        Now it suffices to show that $\sigma^*_{toll} = 0, \sigma^*_{pool}, \sigma^*_{o} = 1 - \sigma^*_{pool}$ satisfy the equilibrium condition \ref{eq: equilibrium condition}.

        Since $\tau > \ugamma$, we know $c^\beta_\gamma(R_{pool}; \sigma) < c^\beta_\gamma(R_{toll}; \sigma)$ for all $\beta \in [0,\ubeta]$ and $\gamma \in [0, \ugamma]$. That is, the cost of paying the HOT toll price will be higher than carpooling for all agents. Hence, nobody will choose $R_{toll}$ and $\sigma^*_{toll} = 0$ satisfies the equilibrium condition \ref{eq: equilibrium condition}. Since $\sigma^*_{toll} + \sigma^*_{pool} + \sigma^*_{o} = 0$, we also have $\sigma^*_{o} = 1 - \sigma^*_{pool}$. 

         An agent $(\beta,\gamma)$ will choose $R_{o}$ over $R_{pool}$ if $c^\beta_\gamma(R_{pool}; \sigma) > c^\beta_\gamma(R_o; \sigma)$, which is equivalent to $\beta < \frac{\gamma}{C_\delta(0, \sigma^*_{pool}, \sigma^*_{o}; \rho)}$. Thus, $R_{o} = \{(\beta, \gamma) : 0 < \beta < \frac{\gamma}{C_\delta(0, \sigma^*_{pool}, \sigma^*_{o}; \rho)} , 0 < \gamma < \ugamma\}$. 

         Since $D = \ubeta \ugamma f(\beta, \gamma)$ and $\sigma^*_{o} = 1 - \sigma^*_{pool}$, the equation \ref{eq:b2-fixed_point2} is equivalent to 
        $$
            \int_{0}^{\ugamma} \int_{0}^{\frac{\gamma}{C_\delta(0, \sigma^*_{pool}, \sigma^*_{o}; \rho)}} f(\beta, \gamma) d\beta d\gamma = \ubeta \ugamma \sigma^*_{o}
        $$

        Therefore, $\sigma^*_{pool}$ and $\sigma^*_{o} = 1 - \sigma^*_{pool}$ satisfies the equilibrium condition \ref{eq: equilibrium condition}.
        
    \end{enumerate}

    \noindent \underline{Regime $B$}: 

        Let $$\sigma_{pool} = \frac{\tau}{2} (\frac{1}{\ugamma - \tau}\sigma_{toll} + \frac{1}{\ugamma})$$ and $$\sigma_{o} = 1 - (\sigma_{toll} + \sigma_{pool}).$$
        First, we need to show that equation \ref{eq:b3-fixed_point}
        $$\left ( 1 - \frac{\tau}{\ubeta C_{\delta}\left(\sigma_{toll}, \sigma_{pool}, \sigma_{o}; \rho\right )}\right) \cdot (\frac{\ugamma - \tau}{\ugamma}) = \sigma_{toll}$$ has a unique fixed point.

        Let $$h(\sigma_{toll}) = \left(1 - \frac{\bar \gamma}{\bar \gamma - \tau} \sigma_{toll}\right)\times C_\delta\left(\sigma_{toll}, \sigma_{pool}, \sigma_{o}; \rho\right).$$

        Then, \begin{align*}
            h(0) = C_\delta\left(0, \frac{\tau}{2\ugamma}, 1- \frac{\tau}{2\ugamma}; \rho\right) > \frac{\tau}{\ubeta}.
        \end{align*}

        Notice also $h(\frac{\ugamma-\tau}{\tau}) = 0$. Since $h$ is continuous and decreasing in $\sigma_{toll}$, there exists a unique  $\sigma^*_{toll}$ such that 
        $$h(\sigma^*_{toll}) = \frac{\tau}{\ubeta},$$
        which is equivalent to equation \ref{eq:b3-fixed_point}.

        Now it suffices to show that $\sigma^*_{toll} = 0, \sigma^*_{pool}, \sigma^*_{o} = 1 - \sigma^*_{pool}$ satisfy the equilibrium condition \ref{eq: equilibrium condition}.
        By comparing the cost functions $c^\beta_\gamma(R_{i}; \sigma)$, we can obtain the best response regions as follow:
        \begin{align*}
            R_{toll} &= \{(\beta, \gamma) : \frac{\tau}{C_\delta(\sigma^*; \rho)} < \beta < \ubeta, \tau < \gamma < \ugamma\}\\
            R_{pool} &= \{(\beta, \gamma) : \frac{\gamma}{C_\delta(\sigma^*; \rho)} < \beta < \ubeta, 0< \gamma < \tau\}\\
            R_{o} &= \{(\beta, \gamma) : 0 < \beta < \frac{\tau}{C_\delta(\sigma^*; \rho)} , \beta C_\delta(\sigma^*; \rho) < \gamma < \ugamma\}
        \end{align*}
        Then, through algebra, we can show that the system
        $$\begin{cases}
        \sigma^*_{toll} &= \left ( 1 - \frac{\tau}{\ubeta C_{\delta}\left(\sigma^*; \rho\right )}\right) \cdot (\frac{\ugamma - \tau}{\ugamma})\\
        \sigma^*_{pool} &= \frac{\tau}{2} (\frac{1}{\ugamma - \tau}\sigma^*_{toll} + \frac{1}{\ugamma})\\
	\sigma^*_{o} &= 1 - (\sigma^*_{toll} + \sigma^*_{pool})
        \end{cases} $$ is equivalent to 
        $$\begin{cases}
        \sigma^*_{toll}D &= \int_{\tau}^{\bar{\gamma}} \int_{\frac{\tau}{C_\delta(\sigma^*; \rho)}}^{\bar{\beta}} f(\beta, \gamma) d\beta d\gamma \\
	\sigma^*_{pool}D &= \int_0^{\tau} \int_{\frac{\gamma}{C_\delta(\sigma^*; \rho)}}^{\bar{\beta}} f(\beta, \gamma) d\beta d\gamma \\
	\sigma^*_{o}D &= \int_0^{\frac{\tau}{C_\delta(\sigma^*; \rho)}} \int_{\beta C_\delta(\sigma^*; \rho)}^{\ugamma} f(\beta, \gamma)  d\gamma d\beta,
        \end{cases}$$
        which completes our proof.
\end{proof}
